# Supplementary material for: QSym$^2$: A Quantum Symbolic Symmetry Analysis Program for Electronic Structure
Source: arXiv:2310.06749 source file (2023-11-30)
Supplement: Supplementary file 5 [file preamble.tex]

% ========
% Preamble
% ========



% ------------------
% Scientific support
% ------------------
% Chemistry
\usepackage[version=4]{mhchem}

% Scientific typesetting
\usepackage{siunitx}
\DeclareSIUnit{\atomicunit}{a.u.}
\DeclareSIUnit\atomicmassunit{u}
\DeclareSIUnit\angstrom{\text {Å}}

% -------------
% Maths support
% -------------
\usepackage{%
  amsthm,%
  amssymb,%
  mathrsfs,%
  mathtools,%
  gensymb,%
  braket,%
  mleftright,%
  nicefrac,%
  interval%
}
\intervalconfig{%
  soft open fences%
}

\mleftright

\newcommand*\bmmax{2}
\usepackage{bm}


% --------
% Diagrams
% --------

% Colours
\usepackage[usenames, svgnames, x11names, rgb]{xcolor}

% Graphics
\usepackage{graphicx}
\usepackage{grffile}

% TikZ & PGFPlots
\usepackage{pgfplots}

% Set up tikzexternalize
\usetikzlibrary{external}
\tikzexternalize
% \tikzexcmd is defined in the compilation call from the command line. See the Makefile.
\newif\iftikzex
\ifdefined\notikzex
  \tikzexfalse
\else
  \tikzextrue
\fi

\iftikzex
  \pgfplotsset{compat=1.18}

  \usetikzlibrary{
    calc,
    luamath,
    positioning,
    decorations.pathreplacing,
    backgrounds,
    arrows.meta,
    pgfplots.groupplots,
    pgfplots.patchplots,
    3d,
  }

  \usepgfplotslibrary[colormaps]

  \pgfplotscreateplotcyclelist{coloronly}{
    {red},
    {blue},
    {black!60!green},
    {black!20!orange},
    {black!30!blue},
    {green!30!brown},
    {blue!40!red},
    {IndianRed},
    {black!40!yellow},
    {Magenta4},
    {DodgerBlue4},
    {Maroon4},
    {Firebrick4},
    {Cyan4},
  }
\fi
\tikzexfalse

% Plot conditionals
\usepackage{xifthen}


% --------
% Captions
% --------
\usepackage{caption, subcaption}


% ------
% Tables
% ------
\usepackage{%
  booktabs,%
  array,%
  adjustbox,%
  makecell,%
  multirow,%
  bigdelim%
}
\newcolumntype{M}[1]{>{\centering\arraybackslash}m{#1}}
\newcolumntype{R}[1]{>{\raggedleft\arraybackslash}m{#1}}

% -----
% Items
% -----
\usepackage[inline]{enumitem}


% --------
% Theorems
% --------
\theoremstyle{plain}
\newtheorem{proposition}{Proposition}
\theoremstyle{remark}
\newtheorem*{remark}{Remark}


% ----------
% Hyperlinks
% ----------
\usepackage[%
  hyperfootnotes=false,%
  hypertexnames=false,%
  hidelinks,%
]{hyperref}
\hypersetup{%
  bookmarksnumbered=true,%
  colorlinks=true,%
  citecolor=teal,%
  linkcolor=Blue4,%
}


% ------------
% Bibliography
% ------------
\usepackage{mciteplus}

% ---------
% Debugging
% ---------
%\listfiles
